# Supplementary material for: Sparse-TDA: Sparse Realization of Topological Data Analysis for Multi-Way Classification
Source: arXiv:1701.03212 ancillary file (2017-11-13)
Supplement: Supplementary file 1 [file Sparse_TDA_supp.pdf]

# Sparse-TDA: Sparse Realization of Topological Data Analysis for Multi-Way Classification

## Supplementary Information

## S.1 Kernel-based TDA Method for Multi-Way Classification

Here, we present the basic terminology of any TDA method by formally defining the mathematical operators and stating the key results. We then use these definitions and results to summarize the multi-scale kernel TDA method. While the kernel TDA method is directly adopted from [? ], we outline it here for the sake of completeness. We also refer the interested reader to Fig. **??** to illustrate how our Sparse-TDA method uses these operators for multi-way classification.

### S.1.1 Terminology

**Filtration:** In computational topology, the "shapes" of data (e.g., point clouds, shapes, images) are frequently described by simplicial (or cubical) complexes. A filtration of a finite simplicial (or cubical) complex $S$ is a sequence of simplicial complexes $S_1, \ldots, S_r$ such that $S_1 \subseteq \ldots \subseteq S_r = S$. A common way to generate a filtration is to consider the sublevel sets $S_t = f^{-1}([-\infty, t])$ of a descriptor function $f : \mathbb{X} \to \mathbb{R}$ on a topological space $\mathbb{X}$ indexed by a parameter $t \in \mathbb{R}$.

**Persistent homology:** As a prevalent tool in TDA, persistent homology is an algebraic approach that quantifies topological features during a filtration of "shapes" [? ? ]. Accordingly, given a topological space $\mathbb{X}$ and a descriptor function $f : \mathbb{X} \to \mathbb{R}$, persistent homology essentially studies the topological changes of the sublevel sets $\mathbb{X}_t = f^{-1}([-\infty, t])$ as $t$ increases from $-\infty$ to $\infty$. During filtration, topological features appear and disappear at different scales that are referred to as the *birth* and *death* times of the features. The short-lived features are considered as noise terms.

**Persistence diagram (PD):** A PD is a concise summary of the topological information captured by persistent homology. From a geometric perspective, the topological features are interpreted as $l$-dimensional holes, e.g., connected components as 0-dimension holes, tunnels as 1-dimensional holes and voids as 2-dimensional holes. Thus, a $l$-dimensional PD is a collection of points in $\mathbb{R}^2$, where each point $(a, b)$ represents a $l$-dimensional hole that is born at time $a$ and filled at time $b$. Fig. **??** illustrates how a filtration from a function $f : \mathbb{R} \to \mathbb{R}$ results in a 0-dimensional PD.

**Stability:** A critical property of PDs is their stability with respect to input noise [? ? ]. A general metric associated with PDs is the *p-Wasserstein distance*, $1 \leq p \leq \infty$. The $p$-Wasserstein distance between the PDs of $f$ and $g$ is defined by

$$d_{W,p}(D_l(f), D_l(g)) = \left( \sum_l \inf_{\gamma_l} \sum_x ||x - \gamma_l(x)||_\infty^p \right)^{\frac{1}{p}}, \quad (1)$$

where the first sum is over all dimensions $l$, the infimum is over all bijections $\gamma_l : D_l(f) \to D_l(g)$ and the second sum is over all points $x \in D_l(f)$ [? ].

Let $X$ be a compact triangulable metric space and $f, g : X \to \mathbb{R}$ be two tame Lipschitz functions with the corresponding PDs $D_l(f)$ and $D_l(g)$ for each dimension $l$. It has been prove that assuming $X$ satisfies a weak condition (see details in [? ]), there exist constants $q \geq 1$ and $C_L$, which

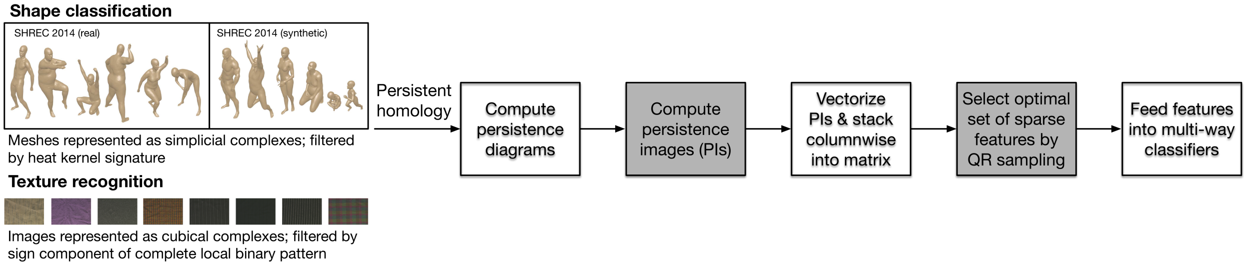


Fig. 1. Pipeline of Sparse-TDA method for multi-way classification. Our contribution lies in linking persistence images with QR pivoting-based sparse sampling, where computational speed-up is realized in both the steps (gray panels).

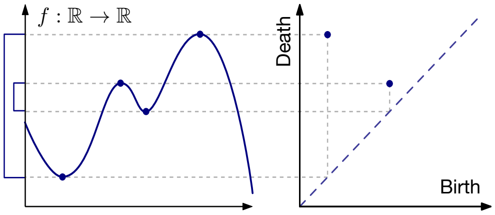


Fig. 2. A function $f : \mathbb{R} \to \mathbb{R}$ (left) and its 0-dimensional PD (right). A connected component in the corresponding sublevel set is created (i.e., birth time) when $t$ passes a new local minimum. As $t$ increases and reaches a local maximum, it merges two connected components (i.e., death time) and is paired with the higher (younger) of the two local minima that represents the two components. The other minimum then represents the connected component resulting from the merger. This figure is adapted from [? ].

depend on $X$ and the Lipschitz constants of $f$ and $g$, such that

$$d_{W,p}(D_l(f), D_l(g)) \le C_L ||f - g||_\infty^{1-\frac{q}{p}}, \; p \ge q. \tag{2}$$

This upper bound on $d_{W,p}(D_l(f), D_l(g))$ implies that a PD $D_l(f)$ is stable with respect to the $p$-Wasserstein distance under small perturbations of $f$.

**Kernel:** Given a set $\mathcal{X}$, $k : \mathcal{X} \times \mathcal{X} \to \mathbb{R}$ is a kernel if there exists a Hilbert space $\mathcal{H}$, called *feature space*, and a map $\Phi : \mathcal{X} \to \mathcal{H}$ such that

$$k(x, x') = \langle \Phi(x), \Phi(x') \rangle_{\mathcal{H}} \tag{3}$$

for all $x, x' \in \mathcal{X}$. In machine learning, a kernel represents a similarity measure between the samples, and $\Phi$ is called its *feature map*. A kernel satisfying Eq. (**??**) is also symmetric and positive definite [? ].

### S.1.2 Multi-scale Kernel TDA

In [? ], Reininghaus et al. develop the *persistence scale space* kernel on the set of PD $\mathcal{D}$ as a multi-scale kernel via a feature map $\Phi_\sigma : \mathcal{D} \to L_2(\Omega)$, where $\Omega = \{x = (x_1, x_2) \in \mathbb{R}^2 : x_2 \ge x_1\}$ denotes the space above the diagonal. Given a PD $D \in \mathcal{D}$, the feature map $\Phi_{\tilde{\sigma}}$ is the solution of a heat diffusion problem with a Dirichlet boundary condition on the diagonal:

$$\Phi_{\tilde{\sigma}}(D) = \frac{1}{4\pi\tilde{\sigma}} \sum_{y \in D} \left( e^{-\frac{||x-y||^2}{4\tilde{\sigma}}} - e^{-\frac{||x-\bar{y}||^2}{4\tilde{\sigma}}} \right), \tag{4}$$

where $\bar{y} = (b, a)$ is the mirror image of $y = (a, b)$ across the diagonal. The map then yields the kernel $k_\sigma : \mathcal{D} \times \mathcal{D} \to \mathbb{R}$ in a closed form as

$$\begin{aligned} k_{\tilde{\sigma}}(F, G) &= \langle \Phi_{\tilde{\sigma}}(F), \Phi_{\tilde{\sigma}}(G) \rangle_{L_2(\Omega)} \\ &= \frac{1}{8\pi\tilde{\sigma}} \sum_{\substack{y \in F \\ z \in G}} \left( e^{-\frac{||y-z||^2}{8\tilde{\sigma}}} - e^{-\frac{||y-\bar{z}||^2}{8\tilde{\sigma}}} \right) \end{aligned} \tag{5}$$

for $\tilde{\sigma} > 0$ and $F, G \in \mathcal{D}$, which has been shown to be 1-Wasserstein stable. Further, note that because the summation in Eq. (**??**) is carried out over all pairwise combinations of the points in the PDs $F$ and $G$, evaluation of the kernel requires $O(|F||G|)$ time, where $|F|$ and $|G|$ denote the number of points in $F$ and $G$, respectively.

## S.2 Additional Results

We run additional experiments with an L1-SVM feature selection method and an L2-regularized linear SVM classifier for our method. The L2-regularized linear SVM is now trained exactly in the same way as the L1-SVM method and implemented using LIBLINEAR. As seen in Fig. **??**, Sparse-TDA outperforms the L1-SVM variants with respect to both classification accuracy and computation time in almost every case. These results further demonstrate the efficiency and effectiveness of QR sampling in our method, and also show the advantage of separating sampling and classification to have greater flexibility in choosing the downstream classifiers. In these experiments, the differentiability of the L2 regularization form helps to solve the optimization problem more easily than the L1 regularization form during training, resulting in higher accuracy and shorter training time.

## References


[S1] J. Reininghaus *et al.*, "A stable multi-scale kernel for topological machine learning," in *Proc. IEEE Conf. Comp. Vis. Pattern Recog. (CVPR 15)*, Boston, MA, June 2015, pp. 4741–4748.

[S2] H. Edelsbrunner *et al.*, "Topological persistence and simplification," *Discrete Comput. Geom.*, vol. 28, no. 4, pp. 511–533, 2002.

[S3] A. Zomorodian and G. Carlsson, "Computing persistent homology," *Discrete Comput. Geom.*, vol. 33, no. 2, pp. 249–274, 2005.

[S4] D. Cohen-Steiner *et al.*, "Stability of persistence diagrams," *Discrete Comput. Geom.*, vol. 37, no. 1, pp. 103–120, 2007.

[S5] ——, "Lipschitz functions have $L_p$-stable persistence," *Found. Comput. Math.*, vol. 10, no. 2, pp. 127–139, 2010.

[S6] L. N. Wasserstein, "Markov processes over denumerable products of spaces, describing large systems of automata," *Problems of Inform. Transmissions*, vol. 5, pp. 47–52, 1969.

[S7] T. Hofmann *et al.*, "Kernel methods in machine learning," *The Ann. of Stat.*, pp. 1171–1220, 2008.

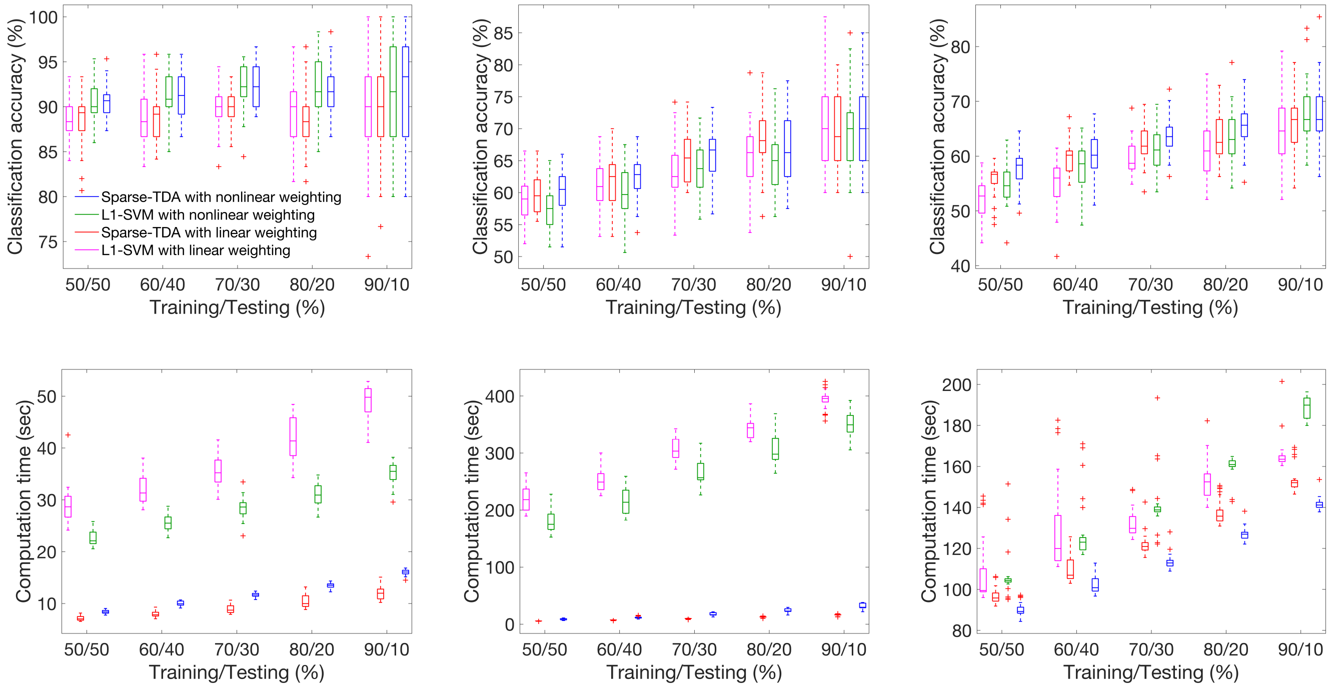


(a) SHREC'14 Synthetic (b) SHREC'14 Real (c) OuTeX Texture

Fig. 3. Comparison of classification accuracy and training time between L1-SVM and Sparse-TDA with a L2-regularized linear SVM classifier for various training-testing data set partition ratios. The results are based on 30 runs in each case.
